# Supplementary material for: Context-aware LLM-based Safe Control Against Latent Risks
Source: arXiv:2403.11863 source file (2025-05-06)
Supplement: Supplementary file 1 [file appendix.tex]

The gradient of the evaluation metric $\nabla_{\param}\myL$ with respect to $\param$ is computed as
\begin{equation} \label{eq:gradient}
    \GradientLshort_{j}(\{R^{[i]}, \boldsymbol{\Phi}^{[i]}, \param^{[i]}\}_{i \in \mathcal{I}}) = \frac{\mathcal{L}(\cdot; \param + \epsilon\cdot \mathbf{e}_j)-\mathcal{L}(\cdot; \param - \epsilon\cdot \mathbf{e}_j)}{2\epsilon},
\end{equation}
where the subscript $j$ is the $j^{\text{th}}$ element of $\nabla_{\param}\mathcal{L}$, $\epsilon$ is the perturbation value, and $\mathbf{e}_{j}$ denotes a vector that takes a scalar value of $1$ in the $j^{\text{th}}$ entry and $0$ otherwise.
